# Supplementary material for: Clifford Circuit Optimization with Templates and Symbolic Pauli Gates
Source: arXiv:2105.02291 source file (2021-11-11)
Supplement: Supplementary file 1 [file appendix.tex]

\appendix
\section{Additional Results on Encoding Circuits for Quantum Error-Correcting Codes}\label{sec:qecc_extra_res}

In this section we present additional details of the performance of the developed methods on the encoding circuit for quantum error-correcting codes~\cite{MarkusCircuits}.

\rs{under construction...}

\begin{figure}
    \centering
    \includegraphics[width=\textwidth, trim=5cm 2cm 5cm 5cm]{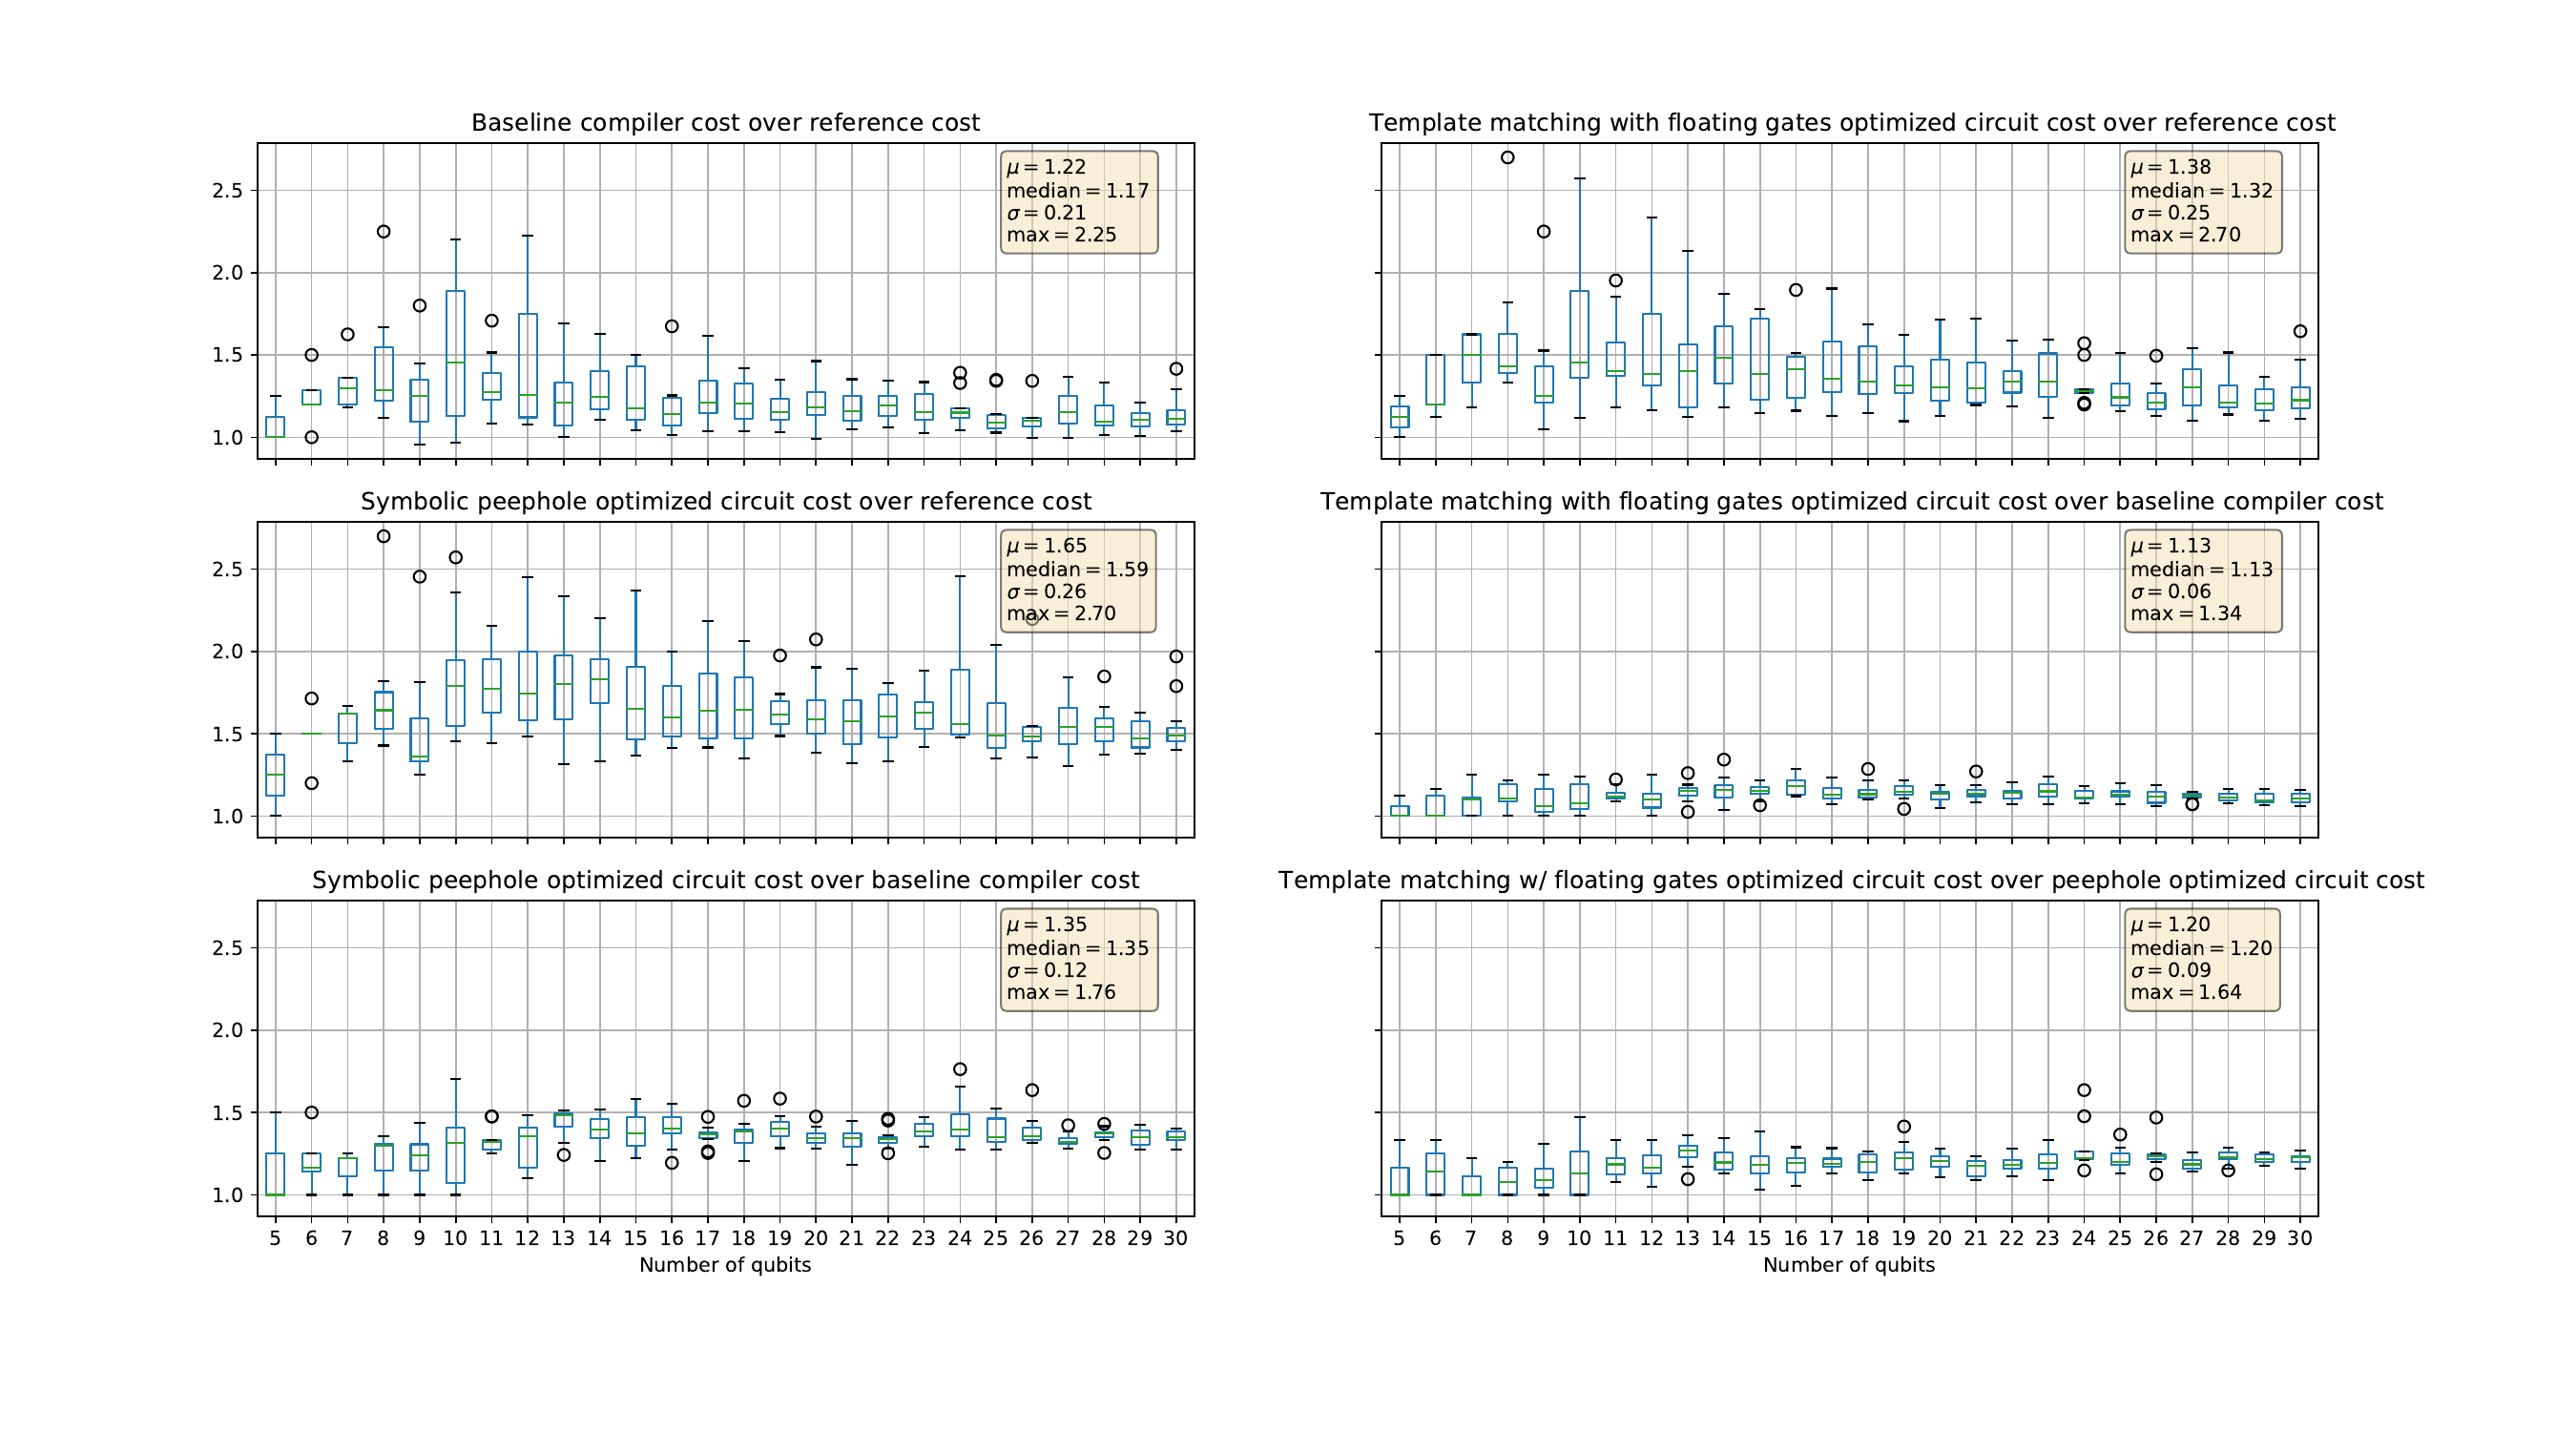}
    \caption{Detailed statistics for the performance of the proposed methods on the encoding circuits for quantum error-correcting codes.}
    \label{fig:qecc_extra_res}
\end{figure}
